# Supplementary material for: On the Granularity of Explanations in Model Agnostic NLP Interpretability
Source: arXiv:2012.13189 source file (2022-08-08)
Supplement: Supplementary file 1 [file save_appendix_segmentation.tex]

\section{Impact of the Segmentation Method on Fidelity}
\label{appendix:segment_experiment}

For GUTEK, we used sentences as elementary units for NLP interpretability. We are interested in a deeper evaluation of the impact of the segmentation on the fidelity, a question we will now explore. We compare the methods TopicTiling~\cite{riedl2012topictiling}, HTMM~\cite{gruber2007htmm} and neural network segmentation~\cite{koshorek2018nnsegment}, referred to hereafter as the \textit{neural} segmentation method.

For the interpretability task of long texts where similar issues as with words may arise with sentences, we thus propose the following experiment. We start with two texts (A and B) of opposite class. We insert a segment from text A into text B, which changes the model output towards the opposite class. We then apply our algorithm to the newly generated text. We know that the inserted segment has a negative effect. We therefore compare the IoU (intersection over union) of the segments with negative effects and extract the segment with highest IoU as the detected segment\footnote{Note that we cannot simply take the most negative segment, since it cannot be guaranteed that the inserted segment is the one with the most negative contribution.}.

Since we have no ground truth segmentation, we use each proposed segmentation method to generate inserts (from A) and insertion points (in B).

For the text segmentation to be of interest, we limit ourselves to long texts of at least 1000 characters.
In addition to the proposed segmentation methods, we add a paragraph segmentation method which simulates prior information. This is done by arranging the created segments as paragraphs in the text. The algorithm therefore \textit{knows} the true segmentation of the text. 
We give the results for the movie review sentiment analysis dataset \cite{panglee2004sentiment}.

The results are given in Table~\ref{table:res_comparison}. Unsurprisingly, truthful prior information cannot be beaten, the paragraph segmentation method performs the best, independently of the ground truth segmentation method. Further, we observe that there seem to be 2 groups of segmentation methods: TopicTiling and the neural method perform well together and HTMM and sentence segmentation perform well together. This is because they produce segments of similar size (See Table~\ref{table:res_complexity_complete} from Appendix~\ref{appendix:segment_length}). This suggests that the segmentation method should be chosen based on the expected size of units to discover, for example topics or paragraphs

We performed experiments on other datasets (20 newsgroups and a custom classification task based on Wikipedia) where results allow to draw the same conclusions as for the movie review dataset.

\begin{table*}[t]
\caption{Comparison of the segmentation methods using IoU. mean(std). Rows: the segmentation methods, Columns: the used ground truth (GT), movie reviews dataset}
\label{table:res_comparison}
\vskip 0.15in
\begin{center}
\begin{small}
\begin{sc}
\begin{tabular}{lcccr}
\toprule
segmentation & Neural GT & TopicTiling GT & Sentence GT & HTMM GT \\
\midrule
Neural      &      0.6(0.34) &          0.41(0.26) &       0.14(0.16) &    0.2(0.21) \\
TopicTiling &     0.37(0.28) &          0.49(0.32) &       0.15(0.14) &   0.23(0.24) \\
HTMM        &     0.22(0.18) &          0.26(0.18) &       0.55(0.45) &   0.48(0.44) \\
Sentence    &     0.14(0.11) &          0.18(0.09) &       0.58(0.48) &   0.44(0.42) \\
Paragraph   &     0.72(0.45) &          0.74(0.43) &       0.54(0.48) &   0.55(0.49) \\
\bottomrule
\end{tabular}
\end{sc}
\end{small}
\end{center}
\vskip -0.1in
\end{table*}

\section{Impact of the Segmentation Method on Segment Length}
\label{appendix:segment_length}
The different segmentation methods produce segments of different lengths. Similar to the analysis in Section~\ref{sec:word-problems:complexity}, we investigate the effect of the different segmentation methods used in Appendix~\ref{appendix:segment_experiment}. The search space for segment based methods is greatly reduced. Instead of being $n_{words}$ dimensional, it is $n_{sentence}$ dimensional. The difference is a factor of $n_{words}/n_{segments}$, the average number of words per segments, which we report in Table~\ref{table:res_complexity_complete}. We also give the time necessary to segment the text, which represents the computational overhead necessary. We observe that they create segments of different length, based on the units to detect. Further, we see a significant difference in segmentation time, representing the computational overhang, with HTMM taking more than 20sec, which of course should be taken into account when reasoning on computation time. Sentence segmentation can however be done in negligible time.

\begin{table*}[t]
\caption{Statistics for the segmentations on the movie review dataset, mean(std). The average text length is 765 words. Movie Reviews Dataset}
\label{table:res_complexity_complete}
\vskip 0.15in
\begin{center}
\begin{small}
\begin{sc}
\begin{tabular}{lcccr}
\toprule
Segmentation & Segments & Words/Segment & Time (sec) \\
\midrule
TopicTiling & 7.1(3.72) & 124.89(59.37) & 0.67(0.3)\\
Neural & 5.19(1.55) & 157.55(78.39) & 0.12(0.05)\\
HTMM & 24.96(10.48) & 31.13(6.1) & 23.33(9.66)\\
Sentence & 35.41(16.13) & 22.47(5.8) & 0.001(0.0004) \\
\bottomrule
\end{tabular}
\end{sc}
\end{small}
\end{center}
\vskip -0.1in
\end{table*}
